# Supplementary material for: Phase equilibrium of water with hexagonal and cubic ice using the SCAN functional
Source: arXiv:2101.04806 ancillary file (2021-01-12)
Supplement: Supplementary file 1 [file PhaseEquilibriumWaterIce.pdf]

# Supplementary information to: Phase equilibrium of water with hexagonal and cubic ice using the SCAN functional

Pablo M. Piaggi,[*,†] Athanassios Z. Panagiotopoulos,[‡,¶] Pablo G. Debenedetti,[‡,¶] and Roberto Car[†,¶,§,‖]

†*Department of Chemistry, Princeton University, Princeton, NJ 08544, USA*

‡*Department of Chemical and Biological Engineering, Princeton University, Princeton, NJ 08544, USA*

¶*Princeton Institute for the Science and Technology of Materials, Princeton University, Princeton, NJ 08544, USA*

§*Department of Physics, Princeton University, Princeton, NJ 08544, USA*

‖*Program in Applied and Computational Mathematics, Princeton University, Princeton, NJ 08544, USA*

E-mail: ppiaggi@princeton.edu

# Contents

**1 MD simulations of TIP4P/Ice** **2**

**2 Crystallization simulations** **3**

**3 Multithermal simulations** **6**

**4 DFT calculations** **7**

**5 Anharmonic effects in ice Ih and ice Ic** **9**

**6 Direct coexistence simulations** **11**

6.1 Preparation of the initial configurations . . . . . . . . . . . . . . . . . . . . . 11

6.2 Ice Ic in NNP-SCAN . . . . . . . . . . . . . . . . . . . . . . . . . . . . . . . 11

6.3 Ice Ih in TIP4P/Ice . . . . . . . . . . . . . . . . . . . . . . . . . . . . . . . . 12

**References** **13**

# 1 MD simulations of TIP4P/Ice

Many of the results reported in the main part of the article are compared to results of TIP4P/Ice. Here we describe the details of the calculations using the TIP4P/Ice model.[1] A cutoff of 8.5 Å was used for the Lennard-Jones and electrostatic interactions. Beyond the cutoff electrostatic interactions were computed using the PPPM method[2] with a relative accuracy in the forces of $10^{-6}$. The effect of the accuracy on the difference in enthalpy between cubic and hexagonal ice at 0 K is analyzed in Figure 1. Tail corrections to the energy and pressure were included. A timestep of 2 fs was used in the coexistence simulations and water molecules were kept rigid using the SHAKE algorithm.[3] The procedure to determine the box size was identical to the one described for the neural network potential (NNP), and the same barostat setup was used. For the energy minimizations a relative error threshold of $10^{-8}$ was used. An energy minimization at constant volume was followed by a minimization with flexible box shape and size.

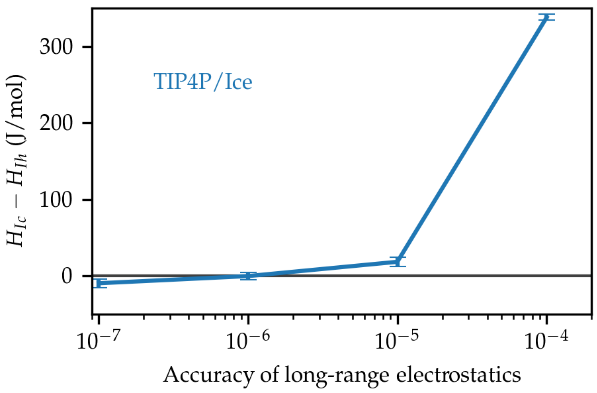


Figure 1: Effect of the relative accuracy of the long range electrostatic energy on the difference in enthalpy between cubic and hexagonal ice at 0 K.

# 2 Crystallization simulations

In Table 1 we report the details of the crystallization simulations used to calculate melting temperatures and differences in chemical potential. Before starting the simulations the box size was set to the average box dimensions in the solid phase. During the simulations an isotropic barostat was used in order to allow for changes in volume relevant to the liquid-solid transformation and to avoid changes in the shape of the box.

Table 1: Computational details of the crystallization simulations. We report the ice polymorph targeted in the simulation, the number of water molecules in the simulation box (# $H_2O$), the temperature or temperature interval targeted, the collective variables (CVs) employed, the number of multiple walker (MWs), the total simulation time per multiple walker, and the enhanced sampling (ES) method used.

| Target ice | # $H_2O$ | Temperature (K) | CVs | MWs | Time (ns) | ES method |
|---|---|---|---|---|---|---|
| Ih | 96 | 300-350 | $E$,$\mathcal{V}$,$s_{Ih}$ | 4 | 73 | OPES |
| Ih | 96 | 350 | $s_{Ih}$ | 4 | 14 | VES |
| Ih | 96 | 340 | $s_{Ih}$ | 4 | 14 | VES |
| Ih | 96 | 330 | $s_{Ih}$ | 4 | 16 | VES |
| Ih | 192 | 350 | $s_{Ih}$ | 4 | 13.5 | VES |
| Ih | 288 | 350 | $s_{Ih}$ | 4 | 23 | VES |
| Ic | 64 | 300-350 | $E$,$\mathcal{V}$,$s_{Ic}$ | 4 | 25 | OPES |
| Ic | 64 | 350 | $s_{Ic}$ | 4 | 15 | VES |
| Ic | 96 | 300-350 | $E$,$\mathcal{V}$,$s_{Ic}$ | 4 | 37 | OPES |
| Ic | 216 | 350 | $s_{Ic}$ | 4 | 42 | VES |
| Ic | 216 | 340 | $s_{Ic}$ | 4 | 28 | VES |

The variationally enhanced sampling (VES)[4] simulations targeted a uniform distribution $p_{\mathrm{tg}(\mathbf{s})}$ and Legendre polynomials of order 40 were used to describe the bias potential. The target distribution and the bias potential were defined in the interval $[0, N]$ where $N$ is the number of molecules in the simulation box. The coefficients in the expansion of the bias potential were optimized using an algorithm similar to stochastic gradient descent[5] with a step size of 2 kJ/mol. We employed four parallel simulations (multiple walkers) that contributed to the statistics to calculate the coefficients. $s_{Ih}$ or $s_{Ic}$ were used as collective variables (CVs). Further details about the VES method can be found in refs. 4 and 6. The crystallization simulations of ice Ih used the same barriers described in ref. 6 to avoid the formation of ice Ic and crystals with undesired orientations. On the other hand, the crystallization simulations of ice Ic did not require any barriers since the formation of ice Ih or undesired structures was not an issue.

The on-the-fly probability enhanced sampling (OPES)[7] simulations employed three CVs, namely the potential energy $E$, the volume $\mathcal{V}$, and either $s_{Ih}$ or $s_{Ic}$. The following expanded ensemble target distribution was used,[7]

$$p_{\mathrm{tg}}(E, \mathcal{V}, s) = \frac{1}{N_\beta} \frac{1}{N_s} \sum_{i=1}^{N_\beta} \sum_{j=1}^{N_s} \frac{e^{-\beta_i (E+P\mathcal{V})+(s-s_j^0)^2/(2\sigma^2)}}{Z_{\beta_i, s_j^0}} \tag{1}$$

where $\beta_i$ with $i = 1, ..., N_\beta$ are inverse temperatures, $s_j^0$ with $j = 1, ..., N_s$ are the centers of umbrella-like distributions, $\sigma$ is the spread of the umbrella-like distributions, and $Z_{\beta_i, s_j^0}$ are the appropriate partition functions. In order to sample the temperature interval $300 - 350$ K we used six equispaced inverse temperatures $\beta_i$ in that interval. $\sigma$ was chosen to be 1.5, and the $s_j^0$ centers were also equispaced in the interval $[0, N]$ with a distance $\sigma$ between them. The bias potential to achieve this distribution is:

$$V(E, \mathcal{V}, s) = -\frac{1}{\beta_0} \log \left( \frac{1}{N_\beta} \frac{1}{N_s} \sum_{i=1}^{N_\beta} \sum_{j=1}^{N_s} e^{(\beta_0 - \beta_i)(E+P\mathcal{V})+(s-s_j^0)^2/(2\sigma^2)+\Delta F_{i,j}} \right), \tag{2}$$

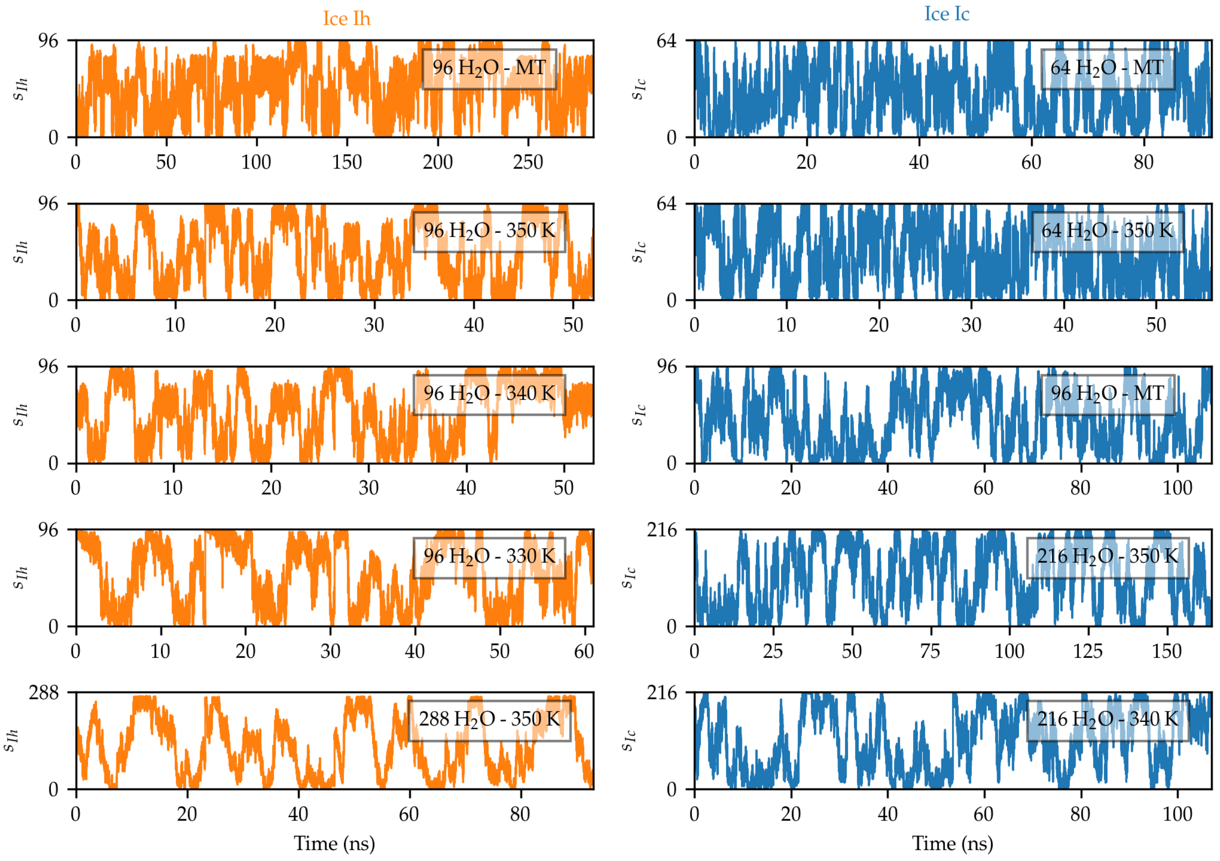


Figure 2: Evolution of $s_{Ih}$ and $s_{Ih}$ as a function of time in the crystallization simulations. The trajectories of the four multiple walkers are concatenated and shown in a single plot.

where $\beta_0$ is the target temperature of the thermostat in the simulation, and $\Delta F_{i,j}$ are free energy differences that have to be determined iteratively as described in ref. 7. The value of $\Delta F_{i,j}$ was updated every 500 MD steps and four multiple walkers contributed to the calculation. The $\Delta F_{i,j}$ converge within a few ns to their final values.

The evolution of $s_{Ih}$ and $s_{Ih}$ as a function of time in the crystallization simulations is shown in Figure 2.

In Figure 1 of the main part, information obtained using small system sizes was used to calculate the melting temperatures of larger systems. We describe here the details of this procedure. For small systems we calculated the difference in chemical potential between ice and water $\Delta\mu$ using multithermal simulations. From these simulations, we obtained continuous information as a function of temperature, i.e. $\Delta\mu(T)$. The results of these

Table 2: Computational details of the multithermal simulations. We report the phase studied, the number of water molecules in the simulation box (# $H_2O$), the temperature or temperature interval targeted, the collective variables (CVs) employed, the number of multiple walkers (MWs), the total simulation time per multiple walker, and the number of different proton configurations used.

| Phase | # $H_2O$ | Temperature (K) | CVs | MWs | Time (ns) | # Proton Confs |
|---|---|---|---|---|---|---|
| Ih | 128 | 100-350 | $E,\mathcal{V}$ | 1 | 8 | 12 |
| Ih | 288 | 260-350 | $E,\mathcal{V}$ | 1 | 4 | 4 |
| Ic | 64 | 100-350 | $E,\mathcal{V}$ | 1 | 13 | 12 |
| Ic | 216 | 260-350 | $E,\mathcal{V}$ | 1 | 2.5 | 4 |
| liquid | 64 | 260-350 | $E,\mathcal{V}$ | 1 | 30 | - |

simulations are shown as continuous lines in Figure 1 of the main part. For larger systems we only calculated $\Delta\mu$ at a few relatively high temperatures. In order to extrapolate these results to lower temperatures we could have fitted a straight line. However, the anomalous behavior of liquid water at low temperatures creates a strong deviation from linear behavior. Thus, we used the function $\Delta\mu(T)$ obtained for smaller systems instead of a straight line. We first fit a spline $f(T)$ to the $\Delta\mu(T)$ obtained for a small system size. Then, we fit $f(T-T^*)$ to the $\Delta\mu$ of a larger system using $T^*$ as a fitting parameter. The results extrapolated in this fashion are shown as dashed lines in Figure 1 of the main part.

# 3 Multithermal simulations

In Table 2 we report the details of the multithermal simulations. We employed the OPES method and the potential energy $E$ and the volume $\mathcal{V}$ as CVs. The target distribution was,

$$p_{\text{tg}}(E,\mathcal{V}) = \frac{1}{N_\beta} \sum_{i=1}^{N_\beta} \sum_{j=1}^{N_s} \frac{e^{-\beta_i(E+P\mathcal{V})}}{Z_{\beta_i}} \tag{3}$$

where $Z_{\beta_i}$ are the appropriate partition functions. Equispaced inverse temperatures $\beta_i$ in the target temperature interval were employed. Simulations targeting the interval $260-350$ K interval used $N_\beta = 20$ while those targeting the interval $100-350$ K used $N_\beta = 26$. Also in this case, the $\Delta F$s were updated every 500 MD steps.

Table 3: Mean and error of the difference in enthalpy between 30 ice Ih and ice Ic structures with different proton configurations calculated using several plane wave kinetic energy cutoffs ($E_c$). The energy was calculated after an optimization of the atomic coordinates and cell vectors.

| $E_c$ | $H_{Ic} - H_{Ih}$ |
|---|---|
| 100 Ry | $99 \pm 8$ |
| 150 Ry | $205 \pm 5$ |
| 200 Ry | $135 \pm 6$ |

# 4 DFT calculations

The wavefunction kinetic energy cutoff in the DFT calculations was chosen to capture the relative stability of ice Ih and ice Ic. In order to do this we calculated the difference in potential energy between a 128-molecule configuration of ice Ih and a 64-molecule configuration of ice Ic ($E_{Ic} - E_{Ih}$) as a function of the wavefunction cutoff. The results are shown in Figure 3. The kinetic energy cutoff for the density was four times larger than the wavefunction kinetic energy cutoff in all cases. The results show that at around 150 Ry the error in the potential energy is around 10 J/mol. This is an acceptable error and for this reason we chose 150 Ry as cutoff for all calculations.

We also performed energy minimizations with respect to the atomic coordinates and cell vectors using several wavefunction cutoffs. We calculated the mean and error of the enthalpy of 30 structures of ice Ih and Ic with different proton configurations. The results are summarized in Table 3 and show that the difference in enthalpy can vary between 99 and 205 J/mol. This is a rather large interval yet the results consistently show that ice Ih is more stable than ice Ic.

We also tested a different pseudopotential parameterized with SCAN instead of with PBE,[8] and found that results did not differ by more than 10 J/mol. Furthermore, we checked the convergence of the energy with respect to the sampling of the Brillouin zone. For this purpose we compared the average energy of 10 ice Ic 64-molecule configurations calculated: 1) using only the gamma point and 2) using a 2x2x2 k-point grid. We found that the results of both calculations were the same within the 5 J/mol error bar. The ice

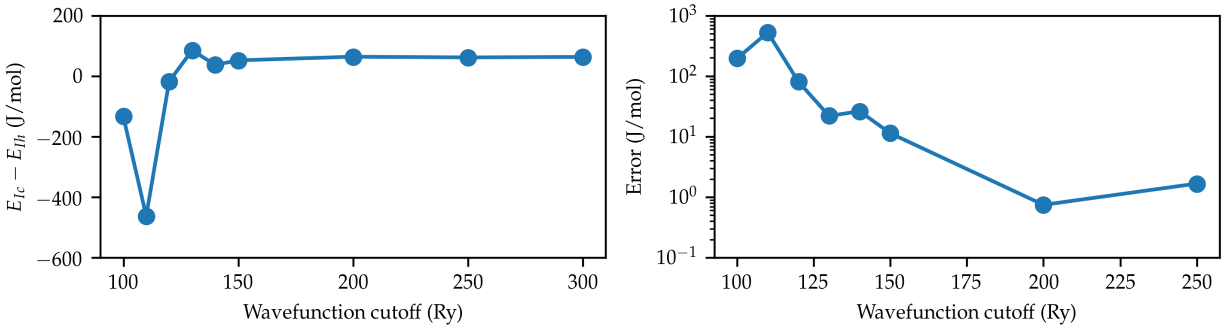


Figure 3: Left) Difference in potential energy between two configurations of ice Ih and ice Ic $E_{Ic} - E_{Ih}$ as a function of the wavefunction cutoff. Right) Error in $E_{Ic} - E_{Ih}$ as a function of the wavefunction cutoff using the value at 400 Ry as reference.

Table 4: Summary of DFT calculations performed on configurations extracted from different simulations driven by the NNP. We report the type of simulation, the phases explored, the number of molecules, the temperature range, the number of proton configurations, the stride for extraction, the total number of configurations used, and other relevant information.

| Simulation | Phase | # $H_2O$ | Temperature (K) | # Proton confs | Stride | Total confs |
|---|---|---|---|---|---|---|
| Crystallization | Ice Ic / Liquid | 64 | 300-350 | - | 25 ps | 4000 |
| Crystallization | Ice Ih / Liquid | 96 | 300-350 | - | 12.5 ps | 18000 |
| Multithermal | Liquid | 64 | 260-350 | - | 25 ps | 1200 |
| Multithermal | Ice Ih | 288 | 260-350 | 4 | 25 ps | 640 |
| Multithermal | Ice Ih | 128 | 100-350 | 12 | 3.125 ps | 28800 |
| Multithermal | Ice Ic | 64 | 100-350 | 12 | 6.25 ps | 25200 |

Ih 128-molecule configurations are bigger than the ice Ic 64-molecule configurations and are thus also converged from the point of view of the sampling of the Brillouin zone.

Configurations were extracted from different simulations driven by the NNP in order to validate the model, and to calculate properties of the DFT model using reweighting. In Table 4 we summarize the simulations that we used, the stride employed for extracting configurations, and the total number of configurations used. The DFT energy was calculated for all these configurations.

In the main part of the article we used the effective sample size (ESS) to quantify the efficiency of the reweighting on DFT energies to calculate chemical potential differences. Here we use the same metric to analyze the efficiency of the calculation of the enthalpies of ice Ih and ice Ic from multithermal simulations driven by the NNP. We show the ESS as a function

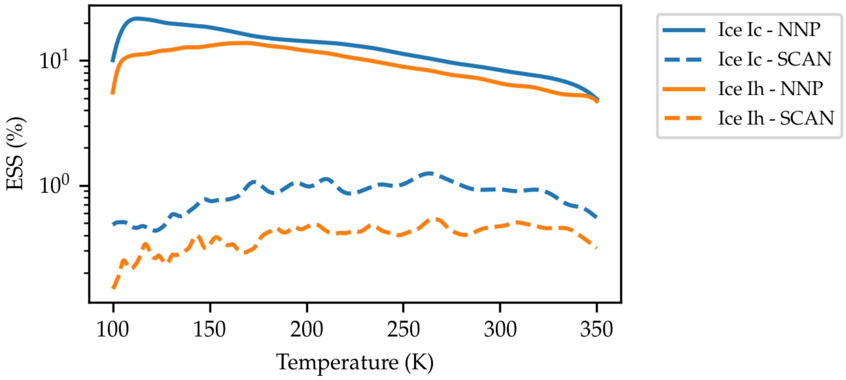


Figure 4: Efficiency of the reweighting of the simulations of ice Ih and ice Ic bewteen 100 and 350 K. The efficiency is calculated using the effective sample size (ESS) expressed as a fraction of the total configurations.

of temperature in Figure 4. The efficiency of the multithermal simulations to calculate properties of the NNP is around 10 % for each temperature, i.e. one in ten configurations is useful for any given temperature in the range 100-350 K. On the other hand, the efficiency of the multithermal simulations to calculate properties of the DFT model is 1 % or lower. This means that only one in one hundred configurations is useful to obtain information at any given temperature.

# 5 Anharmonic effects in ice Ih and ice Ic

We studied the anharmonic contribution to the potential energy and free energy in ice Ih and Ic. The potential energy of a classical solid can be written as

$$E(T) = E_0 + E_{\text{har}}(T) + E_{\text{anh}}(T), \tag{4}$$

where $E_0$ is the energy at 0 K, and $E_{\text{har}}(T)$ and $E_{\text{anh}}(T)$ are the harmonic and anharmonic contributions to the potential energy. $E_{\text{har}}(T)$ is known to be equal to $3nk_BT$ by the equipartition theorem with $n$ the number of atoms in the molecule (for water $n = 3$). We thus computed $E_{\text{anh}}(T) = E(T) - E_0 - E_{\text{har}}(T)$ for ice Ih and Ic using the NNP. The results

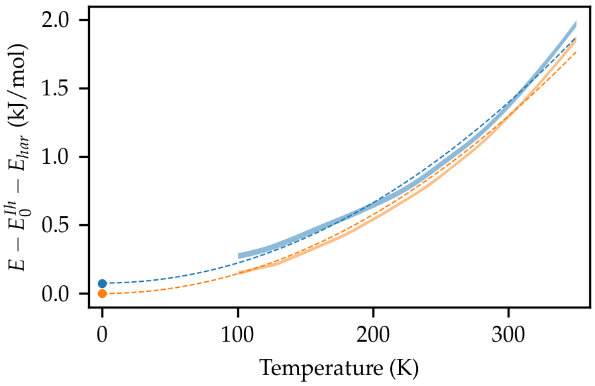


Figure 5: Anharmonic contribution to the potential energy of ice Ih (orange) and ice Ic (blue). The circles are the results at 0 K. The shaded regions are the uncertainties in the determination of the energies at finite temperature. The dashed lines are fits to quadratic functions.

are shown in Figure 5. There is a clear anharmonic component in the potential energy of both polymorphs that is an order of magnitude smaller than its harmonic counterpart. The anharmonic component can be fit reasonably well to a quadratic function $E_{\text{anh}}(T) \approx AT^2$ and we find $A \sim 1.45 \times 10^{-5}$ kJ/mol. The anharmonic effects are the same in ice Ih and Ic within $2 \times 10^{-7}$ kJ/mol. Therefore, in a classical description, we find no stabilization of ice Ih as the one found in ref. 9. Classical SCAN thus predicts that ice Ih is simply stabilized by a lower energy at 0 K.

We can also show that the same result holds for the free energy. The free energy can be written as,

$$G(T) = G_{har}(T) + G_{anh}(T), \tag{5}$$

where $G_{har}(T)$ and $G_{anh}(T)$ are the harmonic and anharmonic contributions, and to a first approximation[10] we write $G_{anh}(T) \approx BT^2$. It can be shown that $B = -A$ and therefore the anharmonic effects obtained for the potential energy will have a similar effect on the free energy.

# 6 Direct coexistence simulations

In the main text we described the results of the direct coexistence simulations between liquid water and ice Ih using the NNP. Here we show the corresponding results for ice Ic, and an application of the same protocol to ice Ih modelled by the TIP4P/Ice potential.

## 6.1 Preparation of the initial configurations

The initial configurations for the coexistence simulations were prepared according to the following procedure. We first performed an MD simulation driven by the NNP in the isothermal-isobaric ensemble of a perfect ice crystal with 288 molecules using an anisotropic barostat. From this simulation we calculated the average lengths, $a$ and $b$, of the simulation box in the directions perpendicular to the interface. We then obtained a liquid configuration with 288 molecules in a box with sides $a$ and $b$. The remaining box length $c$ of the liquid configuration was calculated from a isothermal-isobaric simulation with sides $a$ and $b$ fixed. Next, the solid and liquid configurations were brought together along the direction perpendicular to the sides $a$ and $b$ to form a system of 576 water molecules. We then equilibrated the new system in an isothermal-isobaric simulation in which the sides $a$ and $b$ were fixed but the box length in the direction parallel to the interface was allowed to change to maintain a constant pressure of 1 bar.

## 6.2 Ice Ic in NNP-SCAN

The results of the direct coexistence simulations of liquid water and ice Ic using the NNP based on SCAN are shown in Figure 6. Four simulations with different random seeds for the initial velocities were performed at 307.5 and 310 K. We found that at 307.5 K ice Ic grows and that at 310 K ice Ic melts.

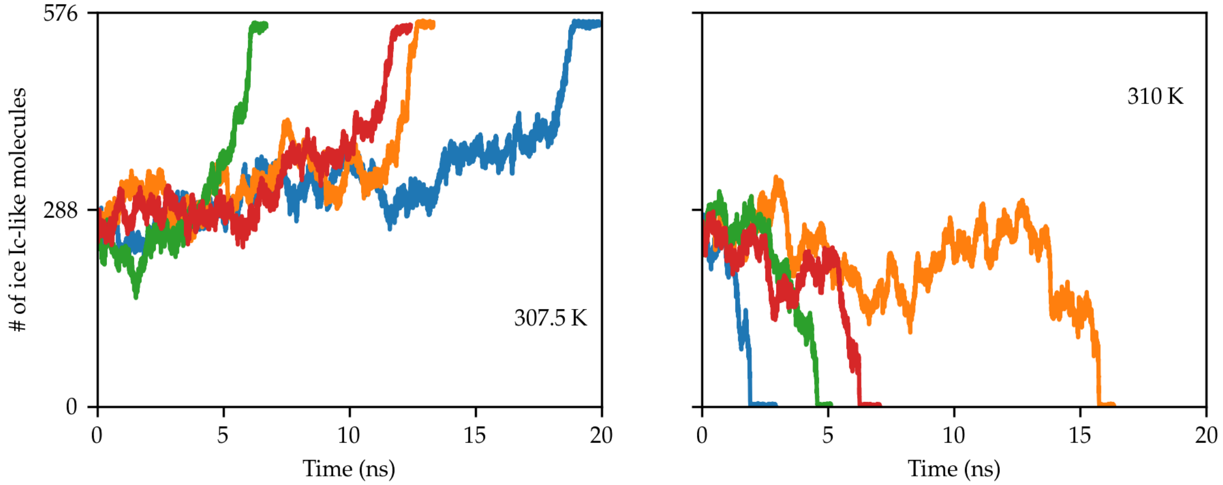


Figure 6: Direct coexistence simulations of liquid water and ice Ic. The number of ice Ic-like molecules[6,11] as a function of simulation time is shown. Four independent runs with different initial seeds for the velocities are shown in different colors at temperatures 307.5 K and 310 K.

## 6.3 Ice Ih in TIP4P/Ice

We performed direct coexistence simulations of liquid water and ice Ih in the TIP4P/model in order to validate the protocol used to calculate the melting temperatures. In these calculations we used a relative accuracy in the long range electrostatic forces of $10^{-4}$. The melting temperature of TIP4P/Ice is well known[6,12] and therefore it is a good test model. The results of the simulations shown in Figure 7. We performed simulations at 265, 266, 267.7, 269, 270 and 275 K with different random seeds for the initial velocities. The evolution of the potential energy per molecule as a function of simulation time is shown in Figure 7. In the range 267.5 to 269 K ice can either grow or melt and it is crucial to perform simulations with different random seeds to rationalize the behavior. This temperature interval where the stochastic behavior is observed is 2 K wide and therefore relatively small. For this reason it was not observed in the coexistence simulations with the NNP. From the direct coexistence simulations we computed the growth probability of the ice Ih slab and we show the results

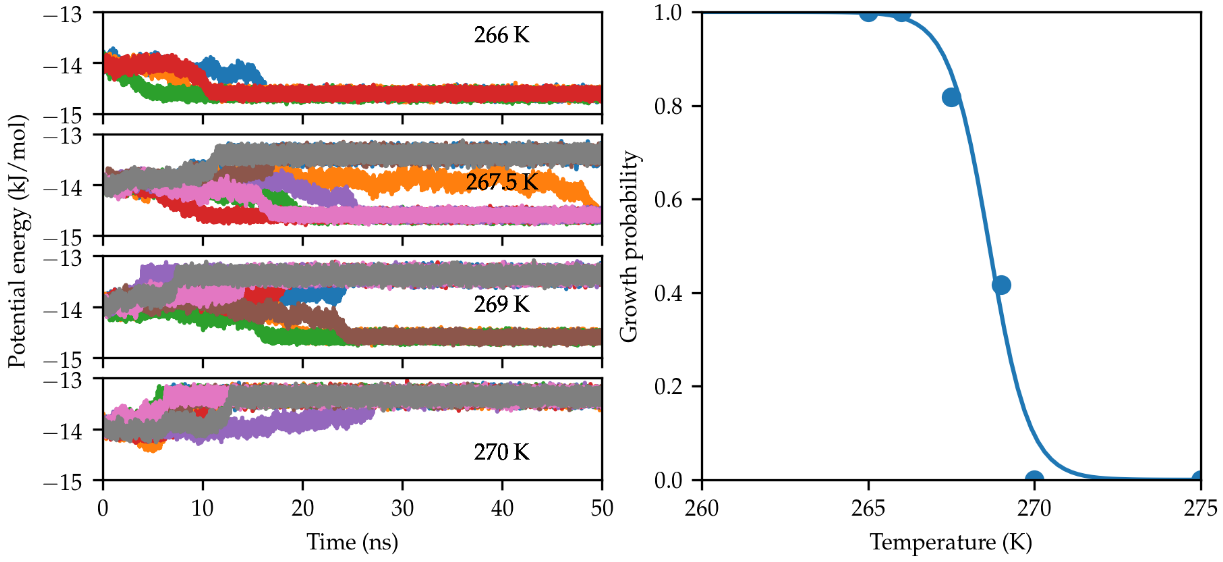


Figure 7: Direct coexistence simulations of liquid water and ice Ih using the TIP4P/Ice model. Left) Potential energy per molecule as a function of time at 266, 267.5, 269, and 270 K. Right) Growth probability as a function of temperature.

in Figure 7. We fit the data to the expression,

$$P(T) = \frac{1}{2} - \frac{1}{2} \tanh\left(\alpha(T - T_m)\right) \tag{6}$$

where $\alpha$ and $T_m$ are the parameters to be determined. We obtained $\alpha = 0.83$ 1/K and $T_m = 269$ K. From this data we estimated the melting temperature to be 269 K in good agreement with the accepted value in the literature (270 K).

# References

(1) Abascal, J.; Sanz, E.; García Fernández, R.; Vega, C. A potential model for the study of ices and amorphous water: TIP4P/Ice. *The Journal of chemical physics* **2005**, *122*, 234511.

(2) Hockney, R. W.; Eastwood, J. W. *Computer simulation using particles*; crc Press, 1988.

(3) Ryckaert, J.-P.; Ciccotti, G.; Berendsen, H. J. Numerical integration of the cartesian

equations of motion of a system with constraints: molecular dynamics of n-alkanes. *Journal of computational physics* **1977**, *23*, 327–341.

(4) Valsson, O.; Parrinello, M. Variational approach to enhanced sampling and free energy calculations. *Physical review letters* **2014**, *113*, 090601.

(5) Bach, F.; Moulines, E. Non-strongly-convex smooth stochastic approximation with convergence rate O (1/n). Advances in Neural Information Processing Systems. 2013; pp 773–781.

(6) Piaggi, P. M.; Car, R. Phase equilibrium of liquid water and hexagonal ice from enhanced sampling molecular dynamics simulations. *The Journal of Chemical Physics* **2020**, *152*, 204116.

(7) Invernizzi, M.; Piaggi, P. M.; Parrinello, M. Unified Approach to Enhanced Sampling. *Phys. Rev. X* **2020**, *10*, 041034.

(8) Yao, Y.; Kanai, Y. Plane-wave pseudopotential implementation and performance of SCAN meta-GGA exchange-correlation functional for extended systems. *The Journal of Chemical Physics* **2017**, *146*, 224105.

(9) Engel, E. A.; Monserrat, B.; Needs, R. J. Anharmonic nuclear motion and the relative stability of hexagonal and cubic ice. *Physical Review X* **2015**, *5*, 021033.

(10) Landau, L. D.; Lifshitz, E. *Statistical physics, part I*; pergamon, Oxford, 1980.

(11) Piaggi, P. M.; Parrinello, M. Calculation of phase diagrams in the multithermal-multibaric ensemble. *The Journal of chemical physics* **2019**, *150*, 244119.

(12) Conde, M.; Rovere, M.; Gallo, P. High precision determination of the melting points of water TIP4P/2005 and water TIP4P/Ice models by the direct coexistence technique. *The Journal of chemical physics* **2017**, *147*, 244506.
